# Supplementary material for: Mutual Information and Optimality of Approximate Message-Passing in Random Linear Estimation
Source: arXiv:1701.05823 source file (2020-08-28)
Supplement: Supplementary file 1 [file appendix_coupledRemainder.tex]

\appendix[Derivation of the coupled remainder] \label{app:Remainder}
The Hamiltonian of this SC perturbed interpolated model is of the form \eqref{eq:int_hamiltonian}, with an appropriate SC periodic matrix $\bm{\phi}$, in which case it can be written as

\begin{align} \label{eq:int_hamiltonian_coupled}
\mathcal{H}_{t,h}(\bx|\mathring{\by}) = \frac{\gamma(t)}{2}\sum_{r=1}^\Gamma \sum_{\mu_r=1}^{M/\Gamma} \Big([\bm{\phi}\bar \bx]_{\mu_r}- \frac{z_{\mu_r}}{\sqrt{\gamma(t)}}\Big)^2 + \frac{\lambda(t)}{2}\sum_{c=1}^\Gamma \sum_{i_c=1}^{N/\Gamma} \Big(\bar x_{i_c}-\frac{\widetilde z_{i_c}}{\sqrt{\lambda(t)}}\Big)^2 + \frac{h}{2}\sum_{c=1}^\Gamma \sum_{i_c=1}^{N/\Gamma} \Big(\bar x_{i_c} - \frac{\widehat z_{i_c}}{\sqrt{h}} \Big)^2,
\end{align}
due to the block structure, where recall that $\{\mu_r\}$ ($\{i_c\}$) is the set of measurement (resp. signal) components indices that belong to the block $r$ (resp. $c$), see section~\ref{sec:deltaopt_deltars}. We now follow the same steps as in section~\ref{sec:partIII}.

As explained in sub-section~\ref{sec:mutualInfoSCmodel_1}, in addition to the observations obtained from the coupled CS model with snr $\gamma(t)$ (first line of \eqref{eq:defChannels} where $\bm{\phi}$ is a periodic matrix, see fig.~\ref{fig:opSpCoupling}), observations about the signal blocks are obtained from $\Gamma$ independent denoising models. We again impose $\gamma(t)$ and $\lambda(t)$ to verify \eqref{eq:boundariesSNR}. Note that the use of a constant trial profile \eqref{eq:constantProfile} implies from \eqref{eq:SEcoupled2}, \eqref{eq:defSigma2} that for any block $c$ we have $\Sigma_c(\tbf{E}; \Delta)^{-2}= \Sigma(E;\Delta)^{-2} = \lambda(0)$ and thus
\be
i^{\rm RS}_{\Gamma,w}(\tbf{E}; \Delta) = i^{\rm RS}(E; \Delta),
\ee
given by \eqref{eq:rs_mutual_info}.
The denoising model associated with the $c$-th block $\bs_c$ of the signal $\bs=[\bs_1, \bs_2, \ldots,\bs_\Gamma]$ is
\be
\widetilde \by_c = \bs_c + \widetilde \bz_c \frac{1}{\sqrt{\lambda(t)}},
\ee
where $\widetilde \bZ_c\sim\mathcal{N}(0,\mathbf{I}_{N/\Gamma})$. With this construction and the use of this constant trial profile note that, similarly as for the non coupled case \eqref{eq:relation_fden_frs}, the MI $i_{\Gamma, w, t,h}^{\rm per}$ of the SC perturbed interpolated model verifies
\begin{align}
i_{\Gamma, w, 0,0}^{\rm per} = i^{\rm RS}(E;\Delta) - \psi(E;\Delta). \label{eq:relation_fden_fr_1}
\end{align}
From this, all the steps \eqref{eq:fundThCalc}-\eqref{eq:lastStepOK} are valid with $i_{t,h}$ replaced by $i^{\rm per}_{\Gamma, w,t,h}$ and $R_{t,h}$ by $R_{w,t,h}$. Equations \eqref{eq:ab}, \eqref{eq:A_twoterms}, \eqref{eq:b} then become 
\begin{align}
\frac{d i^{\rm per}_{\Gamma, w,t,h}}{dt} &= \frac{1}{2L} \sum_{r=1}^\Gamma \mathcal{A}_r +  \frac{1}{2L} \sum_{c=1}^\Gamma\mathcal{B}_c, \label{eq:ab_coup}\\
{\cal A}_r &\defeq \frac{d\gamma(t)}{dt}\sum_{\mu_r=1}^{M/\Gamma} \mathbb{E}\Big[\Big\langle [\bm{\Phi}\bar \bX]_{\mu_r}^2 - \gamma(t)^{-1/2}[\bm{\Phi}\bar \bX]_\mu Z_{\mu_r} \Big\rangle_{t,h}\Big], \label{eq:A_twoterms_coup}\\
{\cal B}_c &\defeq \frac{d\lambda(t)}{dt} \sum_{i_c=1}^{N/\Gamma} \mathbb{E}\Big[\Big\langle \bar X_{i_c}^2 - \lambda(t)^{-1/2}\bar X_{i_c} \widetilde Z_{i_c}\Big\rangle_{t,h}\Big]. \label{eq:b_coup}
\end{align}
Defining naturally the per-block measurement MSE as 
\be
{\rm ymmse}_{r,t,h}\defeq \frac{\Gamma}{M} \sum_{\mu_r=1}^{M/\Gamma}\EE[\langle [\bm{\Phi} \bar \bX]_{\mu_r} \rangle_{t,h}^2 ], \label{eq:ymmserth}
\ee
the previous quantities simplify, after similar integration by parts w.r.t the noise variables like we did for \eqref{eq:was71} and \eqref{eq:was71_2}, to
\begin{align}
\sum_{r=1}^\Gamma \frac{{\cal A}_r}{2L} &=  \frac{d\gamma(t)}{dt}\frac{\alpha B}{2\Gamma}\sum_{r=1}^\Gamma {\rm ymmse}_{r,t,h} = \frac{d\gamma(t)}{dt}\frac{\alpha B}{2\Gamma} \sum_{r=1}^\Gamma\frac{\sum_{c\in r^w} \frac{E_{c,t,h}}{2w+1}}{1+ \gamma(t)\sum_{c\in r^w} \frac{E_{c,t,h}}{2w+1}}, \label{eq:ar} \\
\sum_{c=1}^\Gamma\frac{{\cal B}_c}{2L} &=\frac{d\lambda(t)}{dt} \frac{1}{2\Gamma}\sum_{r=1}^\Gamma E_{r,t,h} = - \frac{d\gamma(t)}{dt}\frac{\alpha B}{2\Gamma} \sum_{r=1}^\Gamma\frac{E_{r,t,h}}{(1+\gamma(t)E)^{2}} = - \frac{d\gamma(t)}{dt}\frac{\alpha B}{2\Gamma} \sum_{r=1}^\Gamma \frac{1}{2w+1} \sum_{c\in r^w} \frac{E_{c,t,h}}{(1+\gamma(t)E)^{2}}, \label{eq:br}
\end{align}
where $\langle-\rangle_{t,h}$ is the posterior expectation associated with the SC perturbed interpolated model. We used \eqref{eq:Ecth} and \eqref{eq:relation_gamma_lambda} for the second equality of \eqref{eq:br} and the periodicity \eqref{eq:eth_long} for the third equality in \eqref{eq:br}. For the second equality in \eqref{eq:ar} we used \eqref{eq:ymmserth_Ecth}. Combining the different pieces together and using \eqref{eq:lastStepOK_0}, \eqref{eq:lastStepOK}, we reach the following remainder which is the counterpart of \eqref{eq:remainder_long} in the SC case
\begin{align}
R_{w,t,h} &= \frac{di^{\rm per}_{\Gamma, w,t,h}}{dt} - \psi(E;\Delta) \\
&= \frac{d\gamma(t)}{dt} \frac{\alpha B}{2\Gamma} \sum_{r=1}^\Gamma \Big(\frac{\sum_{c\in r^w} \frac{E_{c,t,h}}{2w+1}}{1+ \gamma(t)\sum_{c\in r^w} \frac{E_{c,t,h}}{2w+1}} - \frac{\sum_{c\in r^w}\frac{E_{c,t,h}}{2w+1} }{(1+\gamma(t)E)^{2}} -  \frac{E}{1+\gamma(t)E} +\frac{E}{(1+\gamma(t)E)^2}\Big),
\end{align}
which simplifies to \eqref{eq:Rwth} and ends the proof.
