# Supplementary material for: Mutual Information and Optimality of Approximate Message-Passing in Random Linear Estimation
Source: arXiv:1701.05823 source file (2020-08-28)
Supplement: Supplementary file 2 [file appendix_entropy.tex]

\appendix[Recovering the Shannon entropy of $\bS$ from $i^{\rm RS}$ in the noiseless case] \label{app:entropy}
