# Supplementary material for: Mutual Information and Optimality of Approximate Message-Passing in Random Linear Estimation
Source: arXiv:1701.05823 source file (2020-08-28)
Supplement: Supplementary file 3 [file appendix_limit.tex]

\appendix[Existence of the $L\to\infty$ limit of the mutual information] \label{app:limit}
